# Supplementary material for: Active WeaSuL: Improving Weak Supervision with Active Learning
Source: arXiv:2104.14847 source file (2021-04-30)
Supplement: Supplementary file 1 [file 1-dataset.tex]

We used a synthetically generated dataset to investigate the performance of the methods presented in this paper, so that we could better control and explain their behavior. The dataset define by a Gaussian mixture model with discrete latent variables such that we have a hidden class variable that we need to recover. The marginal distribution of the data is given by:

\begin{equation}
    p(x) = \sum_z p(x,z) = \sum_z p(x|z)p(z) = \sum_{k=1}^K \mathcal{N}(x|\mu_k, \Sigma_k) p(z_k = 1)\,
\end{equation}

\noindent
where $K$ is the number of classes. We generate our data by sampling from this distribution using \textit{ancestral sampling}, i.e. first sampling from $p(z)$ and then from $p(x|z)$.

To get a balanced dataset with labels from 2 latent classes, we use $p(z_0 = 1) = p(z_1 = 1) = 0.5$. For the feature distributions we use:
\begin{equation}
    \mu_0 = \begin{bmatrix}
    0.1\\
    1.3
    \end{bmatrix} \hspace{2em}
    \mu_1 = \begin{bmatrix}
    -0.8\\
    -0.5
    \end{bmatrix} \hspace{2em}
    \Sigma_0 = \Sigma_1 = \begin{bmatrix}
    0.25&0\\
    0&0.25
    \end{bmatrix}
\end{equation}

We sample 10,000 points following this procedure. As a result, we get the dataset in figure \ref{fig:synthdataset}:

\begin{figure}[h!]
    \centering
    \includegraphics[width=0.2\linewidth]{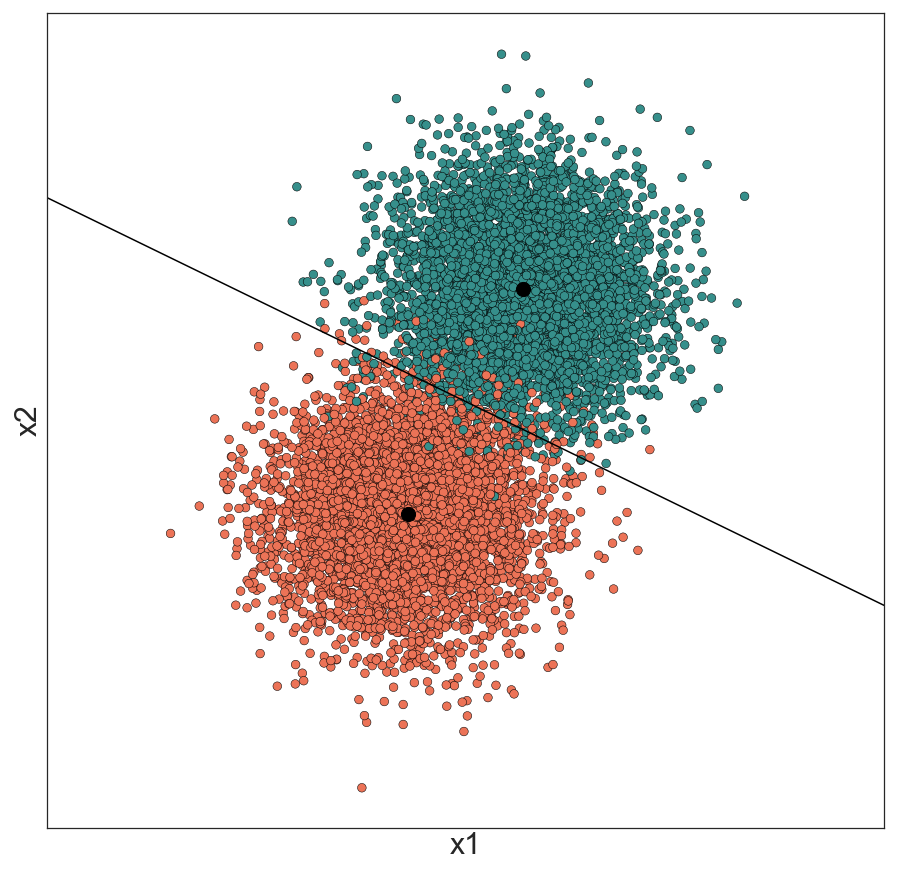}
    \caption{Synthetic dataset}
    \label{fig:synthdataset}
\end{figure}

We create weak labels that divide up the feature space based on the value of one of the features $x_1$ and $x_2$, as shown in figure \ref{fig:wl-synthetic}. The labeling functions that depend on the same features are correlated, so we treat $\lambda_2$ and $\lambda_3$ as a clique in the label model.

\begin{figure}[h!]
    \centering
    \includegraphics[width=\linewidth]{figs/Artboard 27.png}
    \caption{Weak labels for synthetic data}
    \label{fig:wl-synthetic}
\end{figure}
